# Supplementary material for: Revisiting Training Strategies and Generalization Performance in Deep Metric Learning
Source: arXiv:2002.08473 source file (2020-08-01)
Supplement: Supplementary file 1 [file supplementary.tex]

% %%%%%%%% ICML 2020 EXAMPLE LATEX SUBMISSION FILE %%%%%%%%%%%%%%%%%

% \documentclass{article}

% % Recommended, but optional, packages for figures and better typesetting:
% \usepackage{microtype}
% \usepackage{graphicx}
% \usepackage{subcaption}
% \usepackage{booktabs} % for professional tables

% % hyperref makes hyperlinks in the resulting PDF.
% % If your build breaks (sometimes temporarily if a hyperlink spans a page)
% % please comment out the following usepackage line and replace
% % \usepackage{icml2020} with \usepackage[nohyperref]{icml2020} above.
% \usepackage{hyperref}

% % Attempt to make hyperref and algorithmic work together better:
% \newcommand{\theHalgorithm}{\arabic{algorithm}}

% % Use the following line for the initial blind version submitted for review:
% \usepackage{icml2020}

% % If accepted, instead use the following line for the camera-ready submission:
% %\usepackage[accepted]{icml2020}

% % The \icmltitle you define below is probably too long as a header.
% % Therefore, a short form for the running title is supplied here:
% \icmltitlerunning{Supplementary}

% % analyzing deep metric learning: 

% %%%%%%%%%%%%%%%%%%%%%%%%%%%%%%%%%%%%%%%%% CUSTOM PACKAGES
% \usepackage{times}
% \usepackage{epsfig}
% \usepackage{graphicx}
% \usepackage{amsmath}
% \usepackage{amssymb}
% % my packages
% \usepackage[utf8]{inputenc} % allow utf-8 input
% %\usepackage[T1]{fontenc}    % use 8-bit T1 fonts
% %\usepackage{hyperref}       % hyperlinks
% \usepackage{url}            % simple URL typesetting
% \usepackage{booktabs}       % professional-quality tables
% \usepackage{amsfonts}       % blackboard math symbols
% \usepackage{nicefrac}       % compact symbols for 1/2, etc.
% \usepackage{microtype}      % microtypography
% \usepackage{color}
% %\usepackage{subcaption}
% \graphicspath{ {./images/} }
% \usepackage{multirow}
% \usepackage{comment}
% \DeclareMathOperator*{\argmax}{arg\,max}
% \DeclareMathOperator*{\argmin}{arg\,min}



% \newcommand{\red}[1]{\textcolor{red}{#1}}
% \newcommand{\blue}[1]{\textcolor{blue}{#1}}
% \newcommand{\green}[1]{\textcolor{green}{#1}}

% %\newcommand{\best}[1]{\blue{\underline{#1}}}
% \newcommand{\best}[1]{\underline{#1}}

% %%%%%%%%%%%%%%%%%%%%%%%%%%%%%%%%%%%%%%%%% MAIN DOCUMENTS
% \begin{document}
% \onecolumn
% \icmltitle{Supplementary: Revisiting Training Strategies and Generalization Performance in Deep Metric Learning}

% % List of affiliations: The first argument should be a (short)
% % identifier you will use later to specify author affiliations
% % Academic affiliations should list Department, University, City, Region, Country
% % Industry affiliations should list Company, City, Region, Country

% % You can specify symbols, otherwise they are numbered in order.
% % Ideally, you should not use this facility. Affiliations will be numbered
% % in order of appearance and this is the preferred way.
% \icmlsetsymbol{equal}{*}

% \begin{icmlauthorlist}
% \icmlauthor{Aeiau Zzzz}{equal,to}
% \icmlauthor{Bauiu C.~Yyyy}{equal,to,goo}
% \icmlauthor{Cieua Vvvvv}{goo}
% \icmlauthor{Iaesut Saoeu}{ed}
% \icmlauthor{Fiuea Rrrr}{to}
% \icmlauthor{Tateu H.~Yasehe}{ed,to,goo}
% \icmlauthor{Aaoeu Iasoh}{goo}
% \icmlauthor{Buiui Eueu}{ed}
% \icmlauthor{Aeuia Zzzz}{ed}
% \icmlauthor{Bieea C.~Yyyy}{to,goo}
% \icmlauthor{Teoau Xxxx}{ed}
% \icmlauthor{Eee Pppp}{ed}
% \end{icmlauthorlist}

% \icmlaffiliation{to}{Department of Computation, University of Torontoland, Torontoland, Canada}
% \icmlaffiliation{goo}{Googol ShallowMind, New London, Michigan, USA}
% \icmlaffiliation{ed}{School of Computation, University of Edenborrow, Edenborrow, United Kingdom}

% \icmlcorrespondingauthor{Cieua Vvvvv}{c.vvvvv@googol.com}
% \icmlcorrespondingauthor{Eee Pppp}{ep@eden.co.uk}

% % You may provide any keywords that you
% % find helpful for describing your paper; these are used to populate
% % the "keywords" metadata in the PDF but will not be shown in the document
% \icmlkeywords{Machine Learning, ICML}


% % this must go after the closing bracket ] following \twocolumn[ ...

% % This command actually creates the footnote in the first column
% % listing the affiliations and the copyright notice.
% % The command takes one argument, which is text to display at the start of the footnote.
% % The \icmlEqualContribution command is standard text for equal contribution.
% % Remove it (just {}) if you do not need this facility.

% %\printAffiliationsAndNotice{}  % leave blank if no need to mention equal contribution
% % \printAffiliationsAndNotice{\icmlEqualContribution} % otherwise use the standard text.


% %%%%%%%%%%%%%%%%%%%%%%%%%%%%%%%%%%%%%%%%%%%%%%%%%%%%%%%%%%%
% \section{Description of Methods}
% In this section, we briefly describe each DML training objective and triplet mining strategy used in our study, as well as the choice of their individual hyperparameters. General training parameters and details of the training protocol are already discussed in the main paper in Sec. 4.1. For notation, we refer to the embedding of an image $x_i$ including output normalization as $\phi_i=\phi(x_i)$. The non-normalized version is denoted as $\phi^*_i$. All methods operate on the mini-batch $\mathcal{B}$ containing image indices. If not mentioned otherwise, all embeddings operate in dimension $D=128$.
% %%%
% \subsection{Training Criteria}
% \paragraph{Contrastive~\cite{contrastive}} The contrastive training formalism is simple: Given embedding pairs $\mathcal{P}$ (sampled from a mini-batch of size $b$) containing an anchor $\phi_a$ from class $y_a$ and either a positive $\phi_p$ with $y_p=y_a$ or a negative $\phi_n$ from a different class, $y_n\neq y_a$, the network $\phi$ is trained to minimize
% \begin{equation}\label{eq:contrastive}
%     \mathcal{L}_{contr} = \frac{1}{b}\sum^b_{(i,j) \in \mathcal{P}} \mathbb{I}_{y_i=y_j} d_e(\phi_i, \phi_j) + (1-\mathbb{I}_{y_i\neq y_j}) [\gamma - d_e(\phi_i, \phi_j)]_+
% \end{equation}
% with margin $\gamma$, which we set to $1$. The margin ensures that embeddings are not projected arbitrarily far apart from each other. For our distance function we utilize the standard euclidean distance $d_e(x,y) = \left\Vert x-y \right\Vert_2$. We combine the contrastive loss with the distance-weighting negative sampling mentioned below.
% %%%
% \paragraph{Triplet~\cite{face_verfication_inthewild}} Triplets extend the contrastive formalism to provide a concurrent ranking surrogate for both negative and positive sample embeddings using triplets $\mathcal{T}$ sampled from a mini-batch:
% \begin{equation}
%     \mathcal{L}_{tripl} = \frac{1}{b} \sum^{b}_{\substack{(a,p,n)\in\mathcal{T} \\ y_a=y_p\neq y_n}} \left[d_e(\phi_a, \phi_p) - d_e(\phi_a, \phi_n) + \gamma\right]_+
% \end{equation}
% with margin $\gamma=0.2$, thus following recent implementations in e.g. \citet{mic} or \cite{margin}.  Initial works \cite{semihard} using the triplet loss commonly utilized random or semihard triplet sampling and a GoogLeNet-based architecture. Recent methods typically employ the more effective distance-weighted sampling~\cite{margin} and more powerful networks~\cite{mic,Sanakoyeu_2019_CVPR}. For completeness, we compare the triplet-loss performance combinde with random, semihard and distance-weighted sampling schemes introduced below.
% %%%
% \paragraph{Generalized Lifted Structure~\cite{genlifted}}
% The Generalized Lifted Structure loss extends the standard lifted structure loss \cite{lifted} to include all available anchor-positive and anchor-negative distance pairs within a mini-batch $\mathcal{B}$, instead of utilizing only a single anchor-positive combination:
% \begin{equation}
%     \mathcal{L}_{genlift} = \sum_{a\in\mathcal{B}} \left[ \log \sum_{p \in \mathcal{B}, y_a=y_p} \exp{\left(d_e(\phi^*_a, \phi^*_p)\right)} + \log \sum_{n \in \mathcal{B}, y_n \neq y_a} \exp{\left(\gamma-d_e(\phi^*_a,\phi^*_n)\right)}\right]_+ + \frac{\nu}{b}\cdot \sum_{a\in \mathcal{B}} \left\Vert \phi^*_a \right\Vert_2^2 
% \end{equation}

% with mini-batch samples of a class $c$ grouped into $C$, and sets of $C$ contained in $\mathcal{C}$. $\phi^*$ denotes the non-normalized version of $\phi$. The margin $\gamma=1$ serves the standard purpose of avoiding over-distancing already correct image pairs. To account for increasing values, $\nu=0.005$ regularizes the embeddings. 

% \paragraph{N-Pair~\cite{npairs}} N-Pair or N-Tuple losses extend the triplet formalism to incorporate all negatives in the mini-batch $\mathcal{B}$ by
% \begin{equation}
%     \mathcal{L}_{npair} = \frac{1}{b} \sum_{\substack{(a,p) \in \mathcal{B} \\ y_a=y_p, a\neq p}} \log \left(1+\sum_{\substack{n \in \mathcal{B} \\ y_a\neq y_n}} \exp{(\phi_a^{*,T}\phi_n - \phi_a^{*,T}\phi^*_p)}\right) + \frac{\nu}{b}\cdot \sum_{i\in \mathcal{B}} \left\Vert \phi^*_i \right\Vert_2^2 
% \end{equation}
% with embedding regularization $\nu=0.005$, as \cite{npairs} noted a slow convergence for normalized embeddings.
% %%%
% \paragraph{Angular~\cite{angular}}   
% By introducing an angle-based penalty, the angular loss effectively introduces scale invariance and higher-order geometric constraints that are not explicitly introduced in normal contrastive losses:
% \begin{equation}
%     \mathcal{L}_{ang} = \mathcal{L}_{npair}(\phi^*) + \frac{\lambda}{b} \sum_{\substack{(a,p)\in\mathcal{B}\\y_a=y_p, a\neq p}}\left[\log (1+\sum_{\substack{n\in\mathcal{B}\\y_n\neq y_a}} \exp{\left(4\tan^2\left(\alpha(\phi_a + \phi_p)^T\phi_n\right)\right) - 2\left(1+\tan^2(\alpha)\right)\phi_a^T\phi_n} \right] 
% \end{equation}
% with angular margin $\alpha$, which, as proposed in the original paper, is set to $\pi/4$. $\lambda$ is the trade-off between standard ranking losses and the angular constraint.
% %%%
% \paragraph{Arcface~\cite{arcface}}
% Arcface transforms the standard softmax formulation typically used in classification problem to retrieval-based problems by enforcing an angular margin between the embeddings $\phi$ and an approximate center $W\in\mathbb{R}^{c\times d}$ for each class, resulting in 
% \begin{equation}
%     \mathcal{L}_{arc} = -\frac{1}{b}\sum_{i\in\mathcal{B}}\log \frac{\exp(s\cdot\cos{(W_{y_i}^T\phi_i+\gamma=0.5)})}{\exp{(s\cdot\cos{(W_{y_i}^T\phi_i+\gamma=0.5)})} + \sum_{\substack{j\in\mathcal{B}\\y_i\neq y_j}} \exp{(s\cdot\cos{(W_{y_j}^T\phi_i)})}}
% \end{equation}
% Further, this training objective also introduces the additive angular margin penalty $\gamma=0.5$ for increased inter-class discrepancy, while the scaling $s=64$ denotes the radius of the effective utilized hypersphere $\mathbb{S}$. The class centers are optimized with learning rate $0.0005$.
% %%%
% \paragraph{Histogram~\cite{histogram}}
% In contrast to many sample-based ranking objective functions, Histogram Loss learns to minimize the probability of a positive sample pair having a higher similarity score than a negative pair. Given a mini-batch $\mathcal{B}$, the sets of positive similarities $\mathcal{S}^+ = \{\phi_i^T\phi_j | (i,j)\in\mathcal{P}, y_i=y_j\}$ and negative similarities $\mathcal{S}^- = \{\phi_i^T\phi_j | (i,j)\in\mathcal{P},  y_i\neq y_j\}$, one optimises

% \begin{align}
%     \delta(s,r) &= \frac{1}{\Delta} \left(\mathbb{I}_{s\in[t_{r-1},t_r]}\cdot(s-t_{r-1}) + \mathbb{I}_{s\in[t_{r-1},t_r]}\cdot(t_{r+1}-s)\right)\\
%     h^{+/-}(r)    &= \frac{1}{\Vert \mathcal{S}^{+/-} \Vert} \sum_{s\in \mathcal{S}^{+/-}} \delta(s, r)\\
%     \mathcal{L}_{hist} &= \sum_{r\in R} h^-(r) \left( \sum_{q=1}^r h^+(q) \right)
% \end{align}

% resulting in soft, differentiable histogram assignments. The final objective $\mathcal{L}_{hist}$ then penalizes strong overlap between the probability of positive pairs having higher distance (i.e. its cumulative distribution to point $r$) than respective negative pairs.
% Such a histogram loss introduces a single hyperparameter, namely the degree of histogram discretisation $R$, which we set to $51$ for our study. In general, our implementation borrows from the original code base used in \cite{histogram}. 

% \paragraph{Margin~\cite{margin}}
% Margin loss extends the standard triplet loss by introducing a dynamic, learnable boundary $\beta$ between positive and negative pairs. This transfers the common triplet ranking problem to a relative ordering of pairs $\mathcal{P} = \{(i,j) | i,j \in \mathcal{B}, y_i \neq y_j\}$:
% \begin{equation}
%     \mathcal{L}_{margin} = \sum_{(i,j) \in \mathcal{P}} \gamma + \mathbb{I}_{y_i=y_j}(d(\phi_i, \phi_j) - \beta) - \mathbb{I}_{y_i\neq y_j}(d_e(\phi_i, \phi_j)-\beta) 
% \end{equation}
% The learning rate of the boundary $\beta$ is set to $0.0005$, with initial value either $0.6$ or $1.2$ and triplet margin $\gamma=0.2$. For our implementation, we utilise the distance-weighted triplet sampling method highlighted below.
% %%%
% \paragraph{MultiSimilarity~\cite{multisimilarity}}
% Unlike contrastive and triplet based ranking methods, the MultiSimilarity loss concurrently evaluates similarities between anchor and negative, anchor and positive, as well as positive-positive and negative-negative pairs in relation to an anchor:
% \begin{align}
%     s^*_c(i,j) &= \begin{cases}
%                     s_c(\phi_i,\phi_j) \qquad s_c(\phi_i,\phi_j) > \min_{j\in\mathcal{P}_i}s_c(\phi_i,\phi_j) - \epsilon\\
%                     s_c(\phi_i,\phi_j) \qquad s_c(\phi_i,\phi_j) < \max_{k\in\mathcal{N}_i}s_c(\phi_i,\phi_k) + \epsilon\\
%                     0\qquad\qquad\qquad\text{otherwise}
%                     \end{cases}\\
%     \mathcal{L}_{multisim} &= \frac{1}{b} \sum_{i\in \mathcal{B}} \left[ \frac{1}{\alpha}\log[1+\sum_{j\in\mathcal{P}_i}\exp(-\alpha(s^*_c(\phi_i,\phi_j)-\lambda))] + \frac{1}{\beta}\log[1+\sum_{k\in\mathcal{N}_i}\exp(\beta(s^*_c(\phi_i,\phi_k)-\lambda))] \right]
% \end{align}
% where $\mathcal{P}_x$ and $\mathcal{N}_x$ denote the set of positive and negative samples for a sample $x$, with cosine similarity $s_c(x,y) = x^Ty$ for two normalized vectors $x,y\in\mathbb{R}^d$. For our hyperparameters, we use $\alpha=2$, $\beta=40$, $\lambda=0.5$ and $\epsilon=0.1$.
% %%%
% \paragraph{ProxyNCA~\cite{proxynca}}
% The sampling complexity of tuples heavily affects the training convergence. ProxyNCA introduces a remedy by introducing class proxies, which act as approximations to entire classes. This way only an anchor is sampled and compared against the respective positive and negative class proxies. Utilizing one proxy $\psi_c\in\mathbb{R}^d$ per class $c\in\mathcal{C}$, ProxyNCA is then defined as 
% \begin{equation}
%     \mathcal{L}_{proxy} = -\frac{1}{b}\sum_{i\in\mathcal{B}}\log\left(  \frac{\exp(-d_e(\phi_i, \psi_{y_i})}{\sum_{c\in\mathcal{C}\setminus\{y_i\}} \exp(-d(\phi_i, \psi_{c})}  \right)
% \end{equation}
% %%%
% \paragraph{Quadruplet~\cite{quadtruplet}}
% The quadruplet loss is an extension to the triplet loss, which introduces higher level ordering constraint on sample embeddings. By using an anchor, a positive and two exclusive negatives, the quadruplet criterion is defined as:
% \begin{equation}
%     \mathcal{L}_{Quadr} = \sum_{\substack{i,j,k\in\mathcal{B}\\y_i=y_j, y_j\neq y_k}} \left[ d(\phi_i,\phi_j) - d(\phi_i,\phi_k) + \gamma_1 \right]_+ + \sum_{\substack{i,j,k,l\in\mathcal{B}\\y_i=y_j, y_j\neq y_k, y_l\neq y_k, y_l \neq y_j}} \left[ d(\phi_i,\phi_k) - d(\phi_l,\phi_k) + \gamma_2\right]_+
% \end{equation}
% with margin parameters $\gamma_1=1$ and $\gamma_2=0.5$. We utilize distance-weighted sampling to propose the first negative sample $k$, which we found to work better than the quadruplet sampling scheme originally proposed in the paper.
% %%%
% \paragraph{SNR~\cite{signal2noise}} 
% The Signal-to-Noise-Ratio loss (SNR) introduces a novel distance metric based on the ratio between anchor embedding variance and variance of noise, which is simply defined as the difference between anchor and compared embedding. This optimises the embedding space directly for informativeness. The complete loss can then be written as
% \begin{equation}
%     \mathcal{L}_{SNR} = \sum_{i,j,k\in\mathcal{T}} \left[\frac{\sum_{m=1}^D (\phi_{i,m}-\phi_{j,m})}{\sum_{m=1}^D\phi_{i,m}^2} -
%     \frac{\sum_{m=1}^D (\phi_{i,m}-\phi_{k,m})}{\sum_{m=1}^D\phi_{i,m}^2} + \gamma\right]_+ + \frac{\lambda}{b}\sum_{i\in\mathcal{B}}\left\Vert \sum_{m=1}^D\phi_{i,m}\right\Vert
% \end{equation}
% with margin parameter $\gamma=0.2$ and regularization $\lambda=0.005$ to ensure zero-mean distributions. Note that $\phi_{i,m}=\phi(x_i)_m$. 
% %%%
% \paragraph{SoftTriple~\cite{softriple}}
% Similar to ProxyNCA, the SoftTriple objective function utilizes learnable data proxies to tackle the sampling problem. However, instead of class-discriminative proxies, a set of normalized intra-class proxies $\psi \in \Psi^c$ per class $c$ are learned using the NCA-based similarity measure $\mathcal{S}_i^c$ of a sample $i$ to all proxies of a class $c$. Denoting the set of available classes as $\mathcal{C}$ and the total set of proxies as $\Psi$, we get
% \begin{align}
%     \mathcal{S}_i^c      &= \sum_{\psi\in\Psi^c} \frac{\exp(\frac{1}{\gamma}\phi_i^T\psi)}{\sum_{\psi\in\Psi^c} \exp(\frac{1}{\gamma}\phi_i^T\psi)}\\
%     \mathcal{L}_{STBase} &= -\frac{1}{b}\sum_{i\in\mathcal{B}}\log\frac{\exp(\lambda(\mathcal{S}_i^{y_i} - \delta))}{\exp(\lambda(\mathcal{S}_i^{y_i}-\delta)) + \sum_{y\in\mathcal{Y}\setminus \{y_i\}}\exp(\lambda\mathcal{S}_i^{y})}\\
%     \mathcal{L}_{SoftTriple} &= \mathcal{L}_{STBase} + \tau\cdot\frac{\sum_{c\in\mathcal{C}}\sum_{\psi_1,\psi_2\in\Psi^c, \psi_1\neq \psi_2} \sqrt{2 - 2\psi_1^T\psi_2} }{|\mathcal{C}|\cdot|\Psi|\cdot(|\Psi|-1)}
% \end{align}
% The second term denotes a regularization on the learned proxies to ensure sparseness in the class set of proxies. For our tests, we utilised the following hyperparameter values (borrowing from the official implementation in \cite{softriple}): $\tau=0.2$, $\lambda=20$, $\delta=0.01$, $\gamma=0.1$ and the number of proxies per class $|\Psi^c|=10$. The proxy learning rate is set to $0.0005$.
% %%%
% \paragraph{Normalized Softmax~\cite{zhai2018classification}}
% Similar to other classification-based losses in DML that are based on re-formulations of the standard softmax function (such as $\mathcal{L}_{arc}$), the normalized softmax loss is optimized by comparing input embeddings $\phi_i$ to class proxies $\psi\in\mathbb{R}^D$ per class $c\in\mathcal{C}$:
% \begin{equation}
%     \mathcal{L}_{NormSoft} = -\sum_{i\in\mathcal{B}}\log\left( \frac{\exp(\frac{\phi_i^T\psi_{y_i}}{T})}{\sum_{c\in\mathcal{C}\setminus\{y_i\}} \exp(\frac{\phi_i^T\psi_{c}}{T})}\right)
% \end{equation}
% with temperature $T=0.05$ for gradient boosting and class proxy learning rate set to $10^{-5}$.\\ 
% %%%
% \subsection{Tuple Mining}
% Basic contrastive, triplet or higher order ranking losses commonly need to mine their training tuples from the available mini-batch. In our study, we measure the influence of tuple sampling on the standard triplet loss, while utilising Distance-Weighted Mining for all ranking-based objective functions except N-Pair based methods.
% %%
% \paragraph{Random Tuple Mining~\cite{face_verfication_inthewild}}
% The trivial way involves the random sampling of tuples. Simply put, per sample $\{x_i\}_{i\in\mathcal{B}}$ we select a respective positive $\{j | y_j= y_i, i\neq j, j\in\mathcal{B}\}$ or negative sample $\{k |  y_j\neq y_i, i\neq k, k\in\mathcal{B}\}$. 
% %%%
% \paragraph{Semihard Triplet Mining~\cite{semihard}}
% The potential number of triplets scales cubic in training set size. During learning, more and more of those triplets are correctly ordered and effectively provide no training signal \cite{semihard}, thus impairing the remaining training process. To alleviate this, negative samples are carefully selected based on the anchor-positive sample distance (which are sampled at random). Given an anchor embedding $\phi_a$ and its positive $\phi_p$, the negative is sampled randomly from the set 
% \begin{equation}
%     \phi_n \in \{\phi_n | n\in\mathcal{B}, y_n\neq y_a, \left\Vert\phi_a - \phi_p\right\Vert_2^2 < \left\Vert\phi_a - \phi_n\right\Vert_2^2\}. 
% \end{equation}
% This way, only negatives are considered which are reasonably hard to separate from an anchor. Moreover, this mining strategy avoids the sampling of overlay hard negatives, which often correspond to data noise and potentially lead to model collapses and bad local minima~\cite{semihard}.
% %%%
% \paragraph{Distance-Weighted Tuple Mining~\cite{margin}} 
% In DML, the embedding spaces are typically normalized to a $D$-dimensional (unit) hypersphere $\mathbb{S}^{D-1}$ for regularisation purposes \cite{margin}. The analytical distribution of pairwise distances on a hypersphere follows
% \begin{equation}
%     q(d_e(\phi_i,\phi_j)) \propto d_e(\phi_i,\phi_j)^{D-2}[1-\frac{1}{4}d_e(\phi_i,\phi_j)]^{\frac{D-3}{2}}
% \end{equation}

% for arbitrary embedding pairs $\phi_i, \phi_j\in\mathbb{S}^{D-1}$. In order to sample negatives from the whole range of possible distances to an anchor, \citet{margin} propose to sample negatives based on a distance distribution inverse to $q$, i.e.
% \begin{equation}
%     P(n|a) \propto \min(\lambda, q^{-1}(d_e(\phi_a, \phi_n))
% \end{equation}
% We set $\lambda=0.5$ and limit the distances to $1.4$.
% %%%%%


% \subsection{Evaluation Metrics}
% In this section, we examine the evaluation metrics to measure the performance of the studied models on a the testset $\mathcal{X_{\text{test}}}$. 
% \paragraph{Recall@k~\cite{recall}} Let 
% \begin{equation}\label{eq:fk}
% \mathcal{F}_q^k = \argmin_{\mathcal{F}\subset\mathcal{X_{\text{test}}},|\mathcal{F}|=k} \sum_{x_f\in\mathcal{F}} d_e(\phi(x_q),\phi(x_f)) 
% \end{equation}
% be the set of the first $k$ nearest neighbours of a sample $x_p$, then we measure Recall@k as 

% \begin{equation}
%     R@k = \frac{1}{|\mathcal{X_{\text{test}}}|}\sum_{x_q\in\mathcal{X_{\text{test}}}}  
%                 \begin{cases}
%                 1 \qquad \exists \; x_i \in \mathcal{F}_q^k \; \text{s.t.} \; y_i = y_q\\
%                 0 \qquad \text{otherwise}
%                 \end{cases}
% \end{equation}

% which measures the average number of cases in which for a given query $x_q$ there is at least one sample among its top $k$ nearest neighbours $x_i$ with the same class, i.e. $y_i = y_q$.
% %
% \paragraph{Normalized Mutual Information (NMI)~\cite{nmi}} To measure the clustering quality using NMI, we embed all samples $x_i \in \mathcal{X_{\text{test}}}$ to obtain $\Phi_{\mathcal{X_{\text{test}}}}$ and perform a clustering (e.g. $K$-Means \cite{kmeans}). Following, we assign all samples $x_i$ a cluster label $w_i$ indicating the closest cluster center and define $\Omega = \{\omega_k\}_{k=1}^K$ with $\omega_k = \{i | w_i=k\}$ and $K = |\mathcal{C}|$ being the number of classes and clusters. Similarly for the true labels $y_i$ we define $\Upsilon = \{\upsilon_c\}_{c=1}^K$ with $\upsilon_c = \{i | y_i=c\}$. The normalized mutual information is then computed as 
% \begin{equation}
%     NMI(\Omega,\Upsilon) = \frac{I(\Omega,\Upsilon)}{2(H(\Omega) + H(\Upsilon)}
% \end{equation}
% with mutual Information $I(\cdot,\cdot)$ between cluster and labels, and entropy $H(\cdot,\cdot)$ on the clusters and labels respectively.
% %%%
% \paragraph{F1-Score~\cite{npairs}} The F1-score measures the harmonic mean between precision and recall and is a commonly used retrieval metric, placing equal importance to both precision and recall. It is defined as 
% \begin{equation}
%     F1 = \frac{2PR}{P+R}
% \end{equation}
% with precision $P$ and Recall $R$ defined over nearest neighbour retrieval as done for Recall@k.
% %%%
% \paragraph{Mean Average Precision measured on Recall (mAP):} The mAP-score measured on recall follows the same definition as standard mAP. In our case, the mAP is equivalent to the mean over the class-wise average precision@$k_c$ with $k_c$ being the number of samples with label $c \in \mathcal{C}$. With $\mathcal{F}^{k_c}_q$ defined as in eq. \ref{eq:fk}, this gives


% \begin{equation}
%     \text{mAP} = \frac{1}{|\mathcal{X}_{\text{test}}|}\sum_{c\in\mathcal{C}} \sum_{x_q\in \mathcal{X}_{\text{test}} \wedge y_q = c} \frac{\left|\{x_i \in \mathcal{F}^{k_c}_q | y_i=y_q \}\right|}{k_c}
% \end{equation}


% %%%%%%%%%%%%%%%%%%%%%%%%%%%%%%%%%%%%%%%%%%%%%%%%%%%%%%%%%%%%%%%%%%%%
% \section{Correlation between performance and spectral decay $\rho$}
% \input{figures/dists_to_perf}

% Similar to Fig. 5 (rightmost) in the main paper, we now provide a more detailed illustration in Fig. \ref{fig:regularization_effect} comparing the performance of the training objectives and their corresponding spectral decay $\rho(\Phi)$. For ranking losses, we further include the results using $\rho$-regularization while training, which further shows that in each case a gain in performance is related to a decrease of $\rho(\Phi)$. Especially the contrastive loss~\cite{contrastive} greatly profits from our proposed regularization, as also indicated by the analysis of the singular value spectra (cf. Fig. 8 of main paper). Its large gains, more then $5\%$ on the CARS196 dataset, is well explained by comparison of its training objective with those of triplet-based formulations. The latter optimizes over relative positive ($d_\phi(x_a,x_p)$)) and negative distances ($d_\phi(x_a,x_n)$) up to a fixed margin $\gamma$, which counteracts a compression of the embedding space to a certain extend. On the other hand, the constrastive loss, while controlling only the negative distances by $\gamma$, is able to perform an unconstrained contraction of entire classes, which facilitates overly compressed embedding spaces $\Phi$.

% %%%%%%%%%%%%%%%%%%%%%%%%%%%%%%%%%%%%%%%%%%%%%%%%%%%%%%%%%%%%%%%%%%%%
% \section{Analysis of per-class singular value spectra}
% \input{figures/per_class_singular_vector_progression}
% In Sec. 5 of our main paper we analyze generalization in DML by considering the decay of the singular value spectrum over all embedded samples $\Phi_\mathcal{X}$. Thus, we analyze the general compression of the entire embedding space $\Phi$ as unseen test classes can be projected anywhere in $\Phi$, in contrast to \citet{manifoldmixup} which conduct a class-conditioned analysis for i.i.d. classification problems. In order to show that the effect of $\rho$-regularization (as shown in Fig. 8 in main paper) is also reflected in the class-conditioned singular value spectrum, we perform SVD on $\Phi_{y_l}$ and subsequently average over all classes $y_l \in \mathcal{Y}$. Fig. \ref{fig:per_class_singular_value_progression} compares the sorted, first $35$ singular values for both, models trained with and without $\rho$-regularization. We clearly see that the regularization decreases the average decay of singular values similar to the total singular value spectra shown in the main paper.

% %%%%%%%%%%%%%%%%%%%%%%%%%%%%%%%%%%%%%%%%%%%%%%%%%%%%%%%%%%%%%%%%%%%%
% \section{Comparison to state-of-the-art approaches on SOP dataset}
% \input{tables/sota_sop}
% In this section we provide a detailed comparison between current state-of-the-art DML approaches and our strongest baseline model, margin loss (D, $\beta=1.2$)~\cite{margin}, on the SOP dataset in Tab. \ref{tab:eval_sop}. The results for these approaches are taken from their public manuscripts. We observe that our baseline model outperforms each of the models using varying architectures, but especially other ResNet50-based implementations. While R50 proves to be a stronger base network (cf. Fig. 2 of main paper) than GoogLeNet based model, improvements over MIC and D\&C using the same backbone by at least $0.9\%$ and methods based on the similarly strong Inception-BN showcase the relevance of a well-defined baseline. Additionally, even though Rank and ABE employ considerable more powerful network ensembles, our carefully motivated baseline exhibits competitive performance.

% %%%%%%%%%%%%%%%%%%%%%%%%%%%%%%%%%%%%%%%%%%%%%%%%%%%%%%%%%%%%%%%%%%%%
% \section{2D Toy Examples}
% For our toy examples, we use a fully-connected network with two 30 neuron layers. Both input and embedding dimension are 2D, while the latter is normalized onto the unit circle. Each of the four training and test lines contain 15 samples taken from either the diagonal or vertical/horizontal line segments, respectively. We train the networks both with and without regularization for $200$ iterations, a batchsize of $24$ and learning rate of $0.03$ using a standard contrastive loss (eq. \ref{eq:contrastive}) with margin $\gamma=0.1$. For regularisation, we set $p_{\text{switch}}=0.001$.
% Similar to Fig.6 in the main paper, Fig. \ref{fig:straight_toy_example} shows another 2D toy example based on vertical lines which again demonstrates the effect of compression and of our proposed $\rho$-regularization. The example consists of four training lines that are separable only by their $x$-coordinate and a test set of lines which are separable by their $y$-coordinate. As we observe, the test samples are collapsed onto a single point in the non-regularized embedding space, thus can not be distinguished. In contrast, the regularized representation allows us to separate the test classes and, further, exhibits a decreased decay in the singular value spectrum.
% \input{figures/straight_toy_ex}

% %%%%%%%%%%%%%%%%%%%%%%%%%%%%%%%%%%%%%%%%%%%%%%%%%%%%%%%%%%%%%%%%%%%%
% \section{Influence of Manifold Mixup on DML}
% Now, we examine the effect of applying the regularization proposed in ManifoldMixup~\cite{manifoldmixup} on the DML transfer learning setting. As ManifoldMixup has been proposed to increase the compression of a learned representation in the context of standard supervised classification, it is expected to decrease the performance of DML models. For that, we train three different DML models on the CUB200-2011 dataset: (1) Normalized Softmax, (2) Triplet with Distance Sampling and (3) Margin loss with $\beta=0.6$ and Distance Sampling. For (1), the implementation directly follows the standard implementation noted in \citet{manifoldmixup}. For the ranking-based training objectives, we perform mixup in our ResNet50 and generate the mixed class labels, which consequently have either one (if image from the same class are mixed) or two entries (if images from different classes are mixed). Per (mixed) anchor embedding, this gives rise to up to two possible sets of triplets, for which we compute the loss and weigh it by the respective mixup coefficient $\lambda_k$:
% \begin{equation}
%     \mathcal{L}_{tripl}^{\text{Mix}} = \frac{1}{b} \sum_{k=1}^2 \sum^{b}_{\substack{(a,p,n)\in\mathcal{T}^k \\ y_a=y_p\neq y_n}} \lambda_k\cdot\left[d_e(\phi^\lambda_a, \phi^\lambda_p) - d_e(\phi^\lambda_a, \phi^\lambda_n) + \gamma\right]_+
% \end{equation}
% where $\mathcal{T}^k$ denotes the set of triplets given the $k$-th mixup class-label entry and $\lambda_k$ the respective interpolation value. We use the notation $\phi^\lambda_x$ to denote that we now operate on mixup embeddings. For training, we use the standard hyperparameters as described in Sec. 4.1. of the main paper and a mixup-$\alpha$ of $2$ to sample the interpolation values $\lambda\sim\beta(\alpha,\alpha)$ (see \citet{manifoldmixup}).\\
% The results after rerunning baselines and mixup-variants are shown in Fig. \ref{fig:mixup_study}. As expected, applying ManifoldMixup leads to more compressed representations (indicated by a stronger spectral decay and lower $\rho(\Phi)$-scores) at the cost of reduced generalization performance. This holds both for the spectrum across the fully embedded dataset as well as on a class level.

% \input{figures/mixup_study}


% %%%%%%%%%%%%%%%%%%%%%%%%%%%%%%%%%%%%%%%%%%%%%%%%%%%%%%%%%%%%%%%%%%%%
% \section{Detailed Results}
% This section contains the detailed results per method and evaluation metric for the main table of method comparisons (Tab. 2 in the main paper) and the evaluation of batch-creation methods (Fig. 3 in main paper). The corresponding tables for the methods comparisons are Tab. \ref{tab:eval_cub} for CUB200-2011 \cite{cub200-2011}, Tab. \ref{tab:eval_car} for CARS196 \cite{cars196} and Tab. \ref{tab:eval_sop} for Stanford Online Products (SOP) \cite{lifted}. In addition, the switch probability $p_{\text{switch}}$ for each regularised method is noted as well. The batch-creation methods are evaluated in detail in Tab. \ref{tab:meta_sampling_cub} for CUB200-2011, Tab. \ref{tab:meta_sampling_cars} for CARS196 and Tab. \ref{tab:meta_sampling_sop} for SOP. 
% \input{tables/eval_baselines.tex}
% \input{tables/total_comparison.tex}














% \clearpage
% \bibliography{references}
% \bibliographystyle{icml2020}


% \end{document}
